# Supplementary material for: High Information Density and Low Coverage Data Storage in DNA with Efficient Channel Coding Schemes
Source: arXiv:2410.04886 ancillary file (2024-11-11)
Supplement: Supplementary file 1 [file SupplymentaryMaterial_1111.pdf]

# Supplementary Material for: High Information Density and Low Coverage Data Storage in DNA with Efficient Channel Coding Schemes

Yi Ding, Xuan He, Tuan Thanh Nguyen, Wentu Song, Zohar Yakhini, Eitan Yaakobi, Linqiang Pan, Xiaohu Tang, and Kui Cai

# 1 Performance Evaluation and Benchmarking of the Outer ECC Decoder

## 1.1 Performance comparison with state-of-the-art decoders

In prior work [2], the belief propagation (BP) decoding was employed to decode the fountain code (i.e. the Luby Transform (LT) code). However, the BP algorithm has significantly worse performance for decoding Raptor codes due to pre-coding. The Structured Gaussian Elimination (SGE) algorithm, also known as inactivation decoding, is considered the maximum likelihood (ML, i.e., optimal) decoder for decoding fountain codes over erasure channels [3]. In particular, the SGE is able to recover the source data once the received data forms a matrix of full rank. However, in DNA-based data storage channels, limited redundancy in the inner ECC may not adequately detect or correct all the errors, leading to undetectable errors at the output of the inner ECC decoder. Both SGE and BP algorithms cannot address these undetectable errors. Therefore, in this work, we develop a modified basis-finding algorithm (modified-BFA) to decode the fountain codes. Other than the oligo lost, it can also mitigate the erroneously sequences generated by the inner ECC decoder.

We first benchmark the modified BFA algorithm against the SGE algorithm. Compared to standard Gaussian elimination (GE), the SGE retains effectiveness while reducing the computational complexity, especially when the (generator) matrix is sparse. This is achieved by adopting a triangulation operation in the algorithm. In this work, we slightly modify the SGE algorithm by incorporating a reliability ranking. In particular, sequences with larger appearance frequencies during inner ECC decoding are considered more reliable, and SGE is then performed on those more reliable sequences. After ranking, we iteratively examine the list of sequences until an incorrect sequence is identified. Subsequently, SGE is applied to all sequences preceding the incorrect sequence in the ranking as well as to the parity-check matrix of the pre-code. Successful decoding with SGE is achieved if and only if these sequences together with the parity-check matrix form a matrix of full rank. We remark that when the source data is not available, we cannot identify which sequence is the first incorrect one in the ranking list. However, sending the sequences to the SGE decoder one by one for decoding will result in the same successful data recovery rate, at the cost of a higher decoding complexity.

The decoding performance comparison between the modified-BFA and SGE is depicted in Figure S1 and S2. Here, two different inner ECC decoding approaches are applied, namely the “detection” approach and the “decoding” approach. For sequences that do not form valid codewords, the “detection” approach discarded them whereas the “decoding” approach performed decoding on the sequence. In addition, the performance of the BP decoder is also included as a reference. It can be observed that our modified-BFA significantly outperforms both the SGE and BP algorithms.

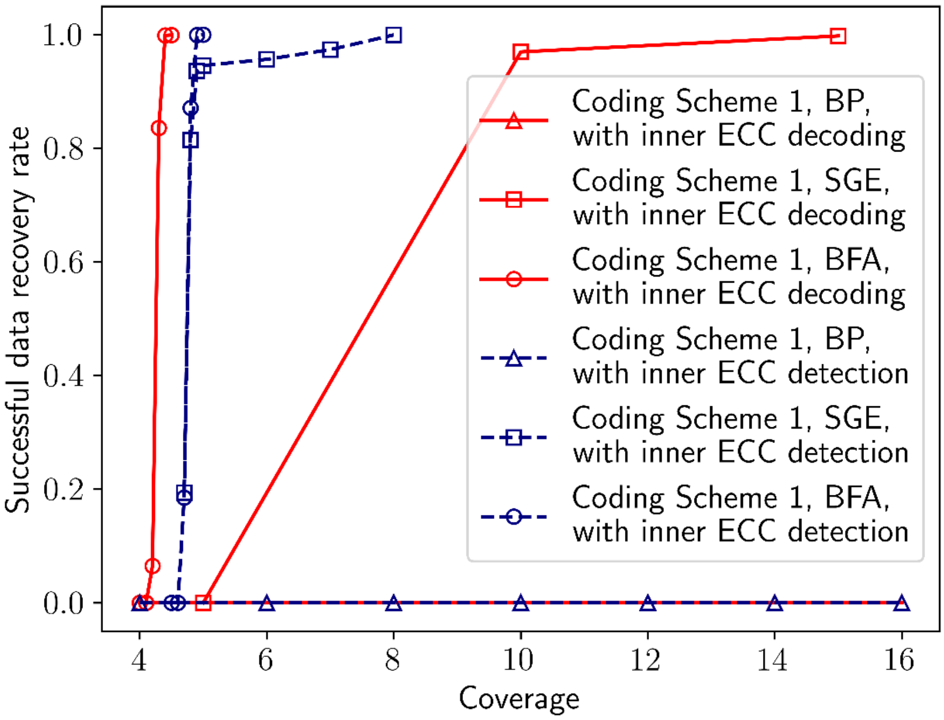


Figure S1: Successful data recovery rate estimated using 1,000 downsampling and data recovery experiments, with different decoding algorithms for Coding Scheme 1.

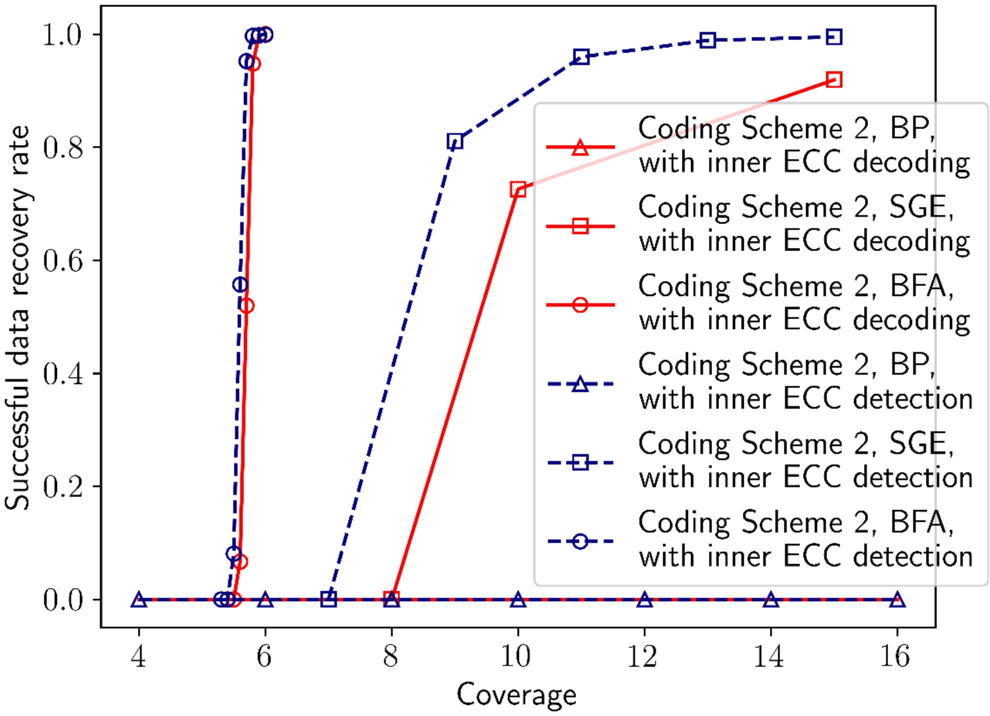


Figure S2: Successful data recovery rate estimated using 1,000 downsampling and data recovery experiments, with different decoding algorithms for Coding Scheme 2.

## 1.2 Benchmarking with an upper bound of outer ECC decoder

An upper bound for the outer ECC decoder can be obtained by performing the SGE exclusively on the correctly received sequences. In this case, the channel is transformed into an erasure channel, where successful decoding solely depends on enough received sequences. This decoder is labeled as “outer ECC UB” in Figures S3 and S4. The comparisons of the performance between the outer ECC upper bound and our modified-BFA algorithm for both Coding Schemes 1 and 2 are depicted in Figures S3 and S4, respectively. These figures demonstrate that our modified-BFA decoder achieves near-optimal performance for both Coding Schemes 1 and 2.

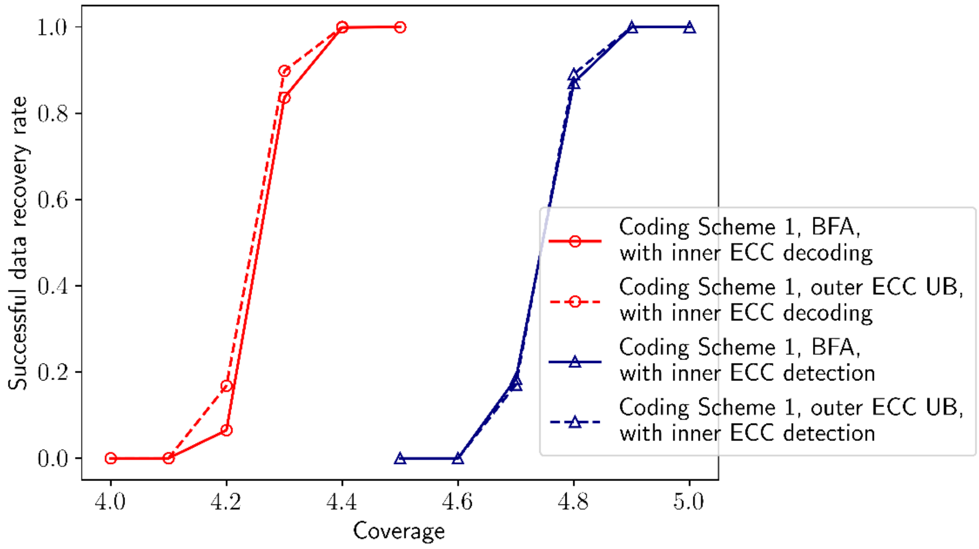


Figure S3: Successful data recovery rate among 1,000 downsampling and data recovery experiments, with BFA and the upper bound for Coding Scheme 1.

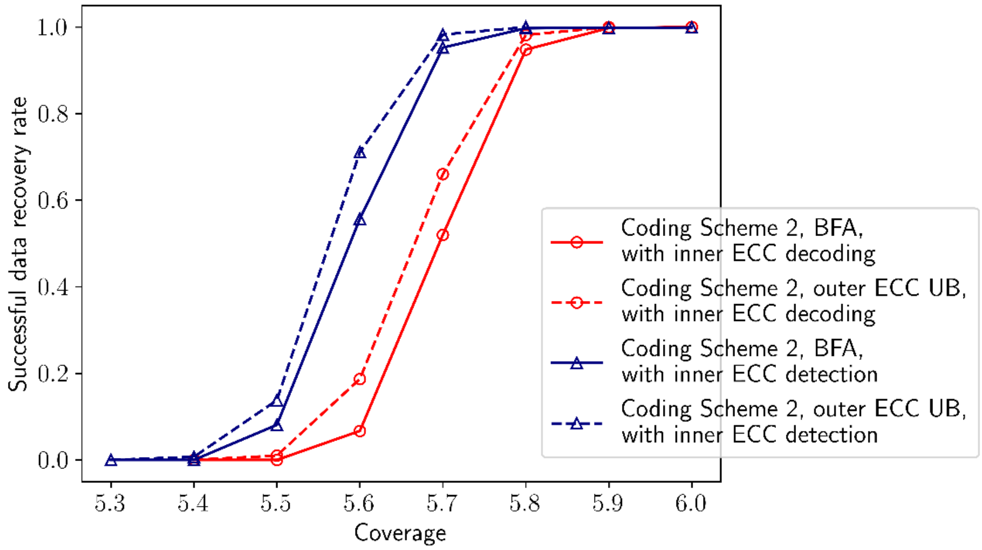


Figure S4: Successful data recovery rate among 1,000 downsampling and data recovery experiments, with BFA and the upper bound for Coding Scheme 2.

## 2 An upper bound for the decoding performance of inner ECC

We specify 'unrecoverable oligos' as the DNA strands/oligos that have either zero reads or one incorrect read. These strands are beyond the recovery capability of any sequence reconstruction algorithm. Let 'unrecoverable oligo rate' denote the ratio of the number of unrecoverable oligos to the number of source oligos, and it indicates the percentage of unrecoverable oligos. It is evident that if the unrecoverable oligo rate exceeds (1 – outer ECC code rate), the outer ECC decoding will inevitably fail. Let $R_1^{out} = 0.95$, and $R_2^{out} = 0.9657$ represent the outer ECC code rates for Coding Schemes 1 and 2, respectively. The simulation results of the unrecoverable oligo rate (Figure S5 and S6) demonstrate that the successful decoding of outer ECC becomes possible only when coverages are at least 4.2 and 5.3 for Coding Scheme 1 and Coding Scheme 2, respectively. These coverage thresholds can be considered the inner ECC's performance upper bounds, as the assumption is that any strands with more than one read can be recovered. Comparing the decoding performance illustrated in Figures S1 and S2 (or Figures S3 and S4), we can observe that there is little room for further enhancement of the inner ECC's performance.

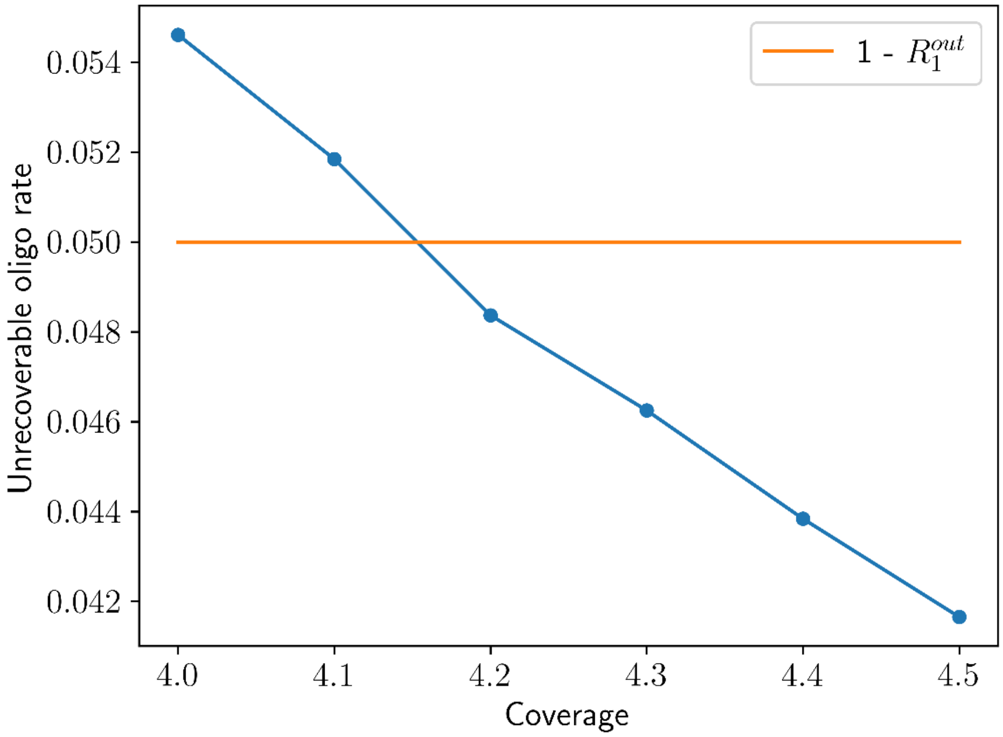


Figure S5: Unrecoverable oligo rates at given coverages for Coding Scheme 1.

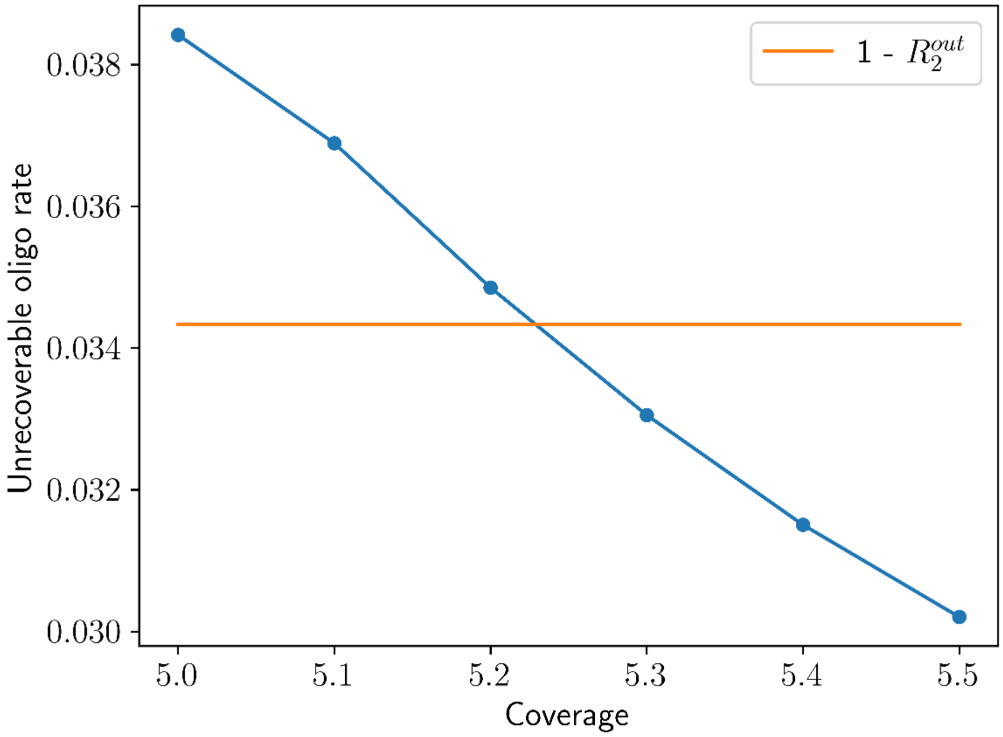


Figure S6: Unrecoverable oligo rates at given coverages for Coding Scheme 2.

## 3 The upper bound of the constrained code rate

In this experiment, each synthesized oligo adhered to the constraints of a homopolymer run length of 3 and a GC content between 45% and 55%. The constrained encoding is carried out in two stages for the data payload part. In the first stage, the modified sequence replacement technique (modified-SRT) introduces a redundancy of 5 nucleotides (nts) to the source sequence to eliminate homopolymer runs longer than 3. In the second stage, the GC-content constraint is imposed through the screening process on a set of candidate oligos generated by the Raptor encoder using different seeds. That is, to generate 30,000 oligos for each coding scheme, a minimum of $\lfloor log_2 30{,}000 \rfloor = 15$ bits are required for the seed. Furthermore, one additional redundant bit is added to create more candidate oligos for screening. Note that this screening process also removes oligos with violation of the homopolymer run length due to the addition of the parity bits of inner ECC, the seed, as well as the coding scheme indicator during subsequence encoding steps after the SRT encoding. In summary, a total of 11 redundant bits are introduced to impose the two biological constraints, leading to a constrained code rate of $2 - \frac{11}{248} = 1.9556$. Motivated by [1], we evaluated the capacity using computational programming, i.e., searching for all sequences satisfying the given constraint through dynamic programming, demonstrating that the capacity is $1.9820$. Therefore, the coding efficiency we achieved is $\frac{1.9556}{1.9820} = 98.67\%$. The most relevant information storage architecture is proposed by [2], which also leverages the features of fountain code to impose the same biological constraints on the encoded oligos. That is, 32 bits are introduced as the seed of the fountain code to generate $72{,}000$ oligos of length 152 nts. While a minimum of 17 bits ($\lceil \log_2 72000 \rceil = 17$) are required for the seed, 15 bits can be considered as the constrained code redundancy. Therefore, the constrained code rate is $2 - \frac{15}{152} = 1.9013$. Considering the code capacity of $1.9806$ for this case [1], the corresponding coding efficiency is $\frac{1.9013}{1.9806} = 96.00\%$. It represents the highest coding efficiency achieved by all prior experimental works. In this work, both our Coding Schemes 1 and 2 outperform it.

Furthermore, in [2], both the homopolymer runlength constraint and the GC-content constraint are imposed though the screening processing, resulting in a low screening pass rate of 16% [1], and thereby a high encoding latency. Since the homopolymer runlength constraint is a strong deterministic constraint, in this work, for the data payload part, we carry out the corresponding constrained encoding separately based on SRT, and only the GC-content constraint is ensured by screening. Correspondingly, 50,718 and 39,438 times encoding are conducted to successfully generate 30,000 oligos for Coding Schemes 1 and 2, respectively. It leads a screening pass rate of 59.19% and 76.07%. Therefore, the encoding latency is also significantly reduced.

## Reference


[1] Liu, Y. He, X. Tang, X. "Capacity-Achieving Constrained Codes with GC-Content and Runlength Limits for DNA Storage," *2022 IEEE International Symposium on Information Theory (ISIT)*, Espoo, Finland, 2022, pp. 198-203.

[2] Erlich, Y. Zielinski, D. "DNA Fountain enables a robust and efficient storage architecture." science 355.6328 (2017): 950-954.

[3] Shokrollahi, A. & Luby, M. Raptor codes. Foundations and Trends® in Communications and Information Theory 6, 213–322 (2011).
